# Supplementary material for: Synthetic supply networks
Source: arXiv:2608.03716 source file (2026-08-04)
Supplement: Supplementary file 1 [file supplementary.tex]

documentclass[11pt]{article} %uncomment for standalone .tex
\input{packages.tex} %uncomment for standalone .tex
\begin{document} %uncomment for standalone .tex
\appendix 

\tableofcontents

\input{supplementary_body.tex}

% uncomment for standalone .tex
\newpage
% Bibliography
\small
\renewcommand\bibname{References}
\bibliographystyle{unsrtnat}
\bibliography{bib}
\normalsize

\end{document} %uncomment for standalone .tex
